# Supplementary material for: Machine Theory of Mind for Autonomous Cyber-Defence
Source: arXiv:2412.04367 source file (2024-12-05)
Supplement: Supplementary file 1 [file gido.tex]

\section{\gido results} \label{appendix:gido:results}

\subsection*{Convergence Plots for \gido} \label{appendix:gido:results:convergence_plots}

\begin{figure}[H]
\centering
\includegraphics[width=0.9\columnwidth]{./experiments/RedHVTPreferenceSPDeterministic/BlueMSNDeterministic/TreeNetwork30/results/report_plots/gido/convergence_plots_legend.pdf}

\subfloat[\treeThirty]{
\label{fig:RedHVTPreferenceSPDeterministic:BlueMSNDeterministic:TreeNetwork30:convergence_plots:gido}
\includegraphics[width=0.9\columnwidth]{./experiments/RedHVTPreferenceSPDeterministic/BlueMSNDeterministic/TreeNetwork30/results/report_plots/gido/convergence_plots.pdf}
}

\subfloat[\treeForty]{
\label{fig:RedHVTPreferenceSPDeterministic:BlueMSNDeterministic:TreeNetwork40:convergence_plots:gido}
\includegraphics[width=0.9\columnwidth]{./experiments/RedHVTPreferenceSPDeterministic/BlueMSNDeterministic/TreeNetwork40/results/report_plots/gido/convergence_plots.pdf}
}

\subfloat[\treeFifty]{
\label{fig:RedHVTPreferenceSPDeterministic:BlueMSNDeterministic:TreeNetwork50:convergence_plots:gido}
\includegraphics[width=0.9\columnwidth]{./experiments/RedHVTPreferenceSPDeterministic/BlueMSNDeterministic/TreeNetwork50/results/report_plots/gido/convergence_plots.pdf}
}

\subfloat[\treeSeventy]{
\label{fig:RedHVTPreferenceSPDeterministic:BlueMSNDeterministic:TreeNetwork70:convergence_plots:gido}
\includegraphics[width=0.9\columnwidth]{./experiments/RedHVTPreferenceSPDeterministic/BlueMSNDeterministic/TreeNetwork70/results/report_plots/gido/convergence_plots.pdf}
}

\subfloat[\treeNinety]{
\label{fig:RedHVTPreferenceSPDeterministic:BlueMSNDeterministic:TreeNetwork90:convergence_plots:gido}
\includegraphics[width=0.9\columnwidth]{./experiments/RedHVTPreferenceSPDeterministic/BlueMSNDeterministic/TreeNetwork90/results/report_plots/gido/convergence_plots.pdf}
}

\subfloat[\treeMixed]{
\label{fig:RedHVTPreferenceSPDeterministic:BlueMSNDeterministic:TreeNetworkMixed:convergence_plots:gido}
\includegraphics[width=0.9\columnwidth]{./experiments/RedHVTPreferenceSPDeterministic/BlueMSNDeterministic/TreeNetworkMixed/results/report_plots/gido/convergence_plots.pdf}
}

\caption{Convergence plots from our \tree runs. For each set of plots a \gido was trained data gathered on the respective \tree topology using \blueMSND and
\redHVTPreferenceSP agents.}
\label{fig:treenets:convergence:gido}
\end{figure}

\subsection*{High-Value Target Confusion Matrices for \gido} \label{appendix:gido:results:hvt_cm}

\begin{figure}[H]
    \centering

    \subfloat[\treeThirty]{
    \label{fig:RedHVTPreferenceSPDeterministic:BlueMSNDeterministic:TreeNetwork30:hvt_CMs:gido}
    \includegraphics[width=0.8\columnwidth]{./experiments/RedHVTPreferenceSPDeterministic/BlueMSNDeterministic/TreeNetwork30/results/report_plots/gido/hvt_CMs.pdf}
    }

    \subfloat[\treeForty]{
    \label{fig:RedHVTPreferenceSPDeterministic:BlueMSNDeterministic:TreeNetwork40:hvt_CMs:gido}
    \includegraphics[width=0.8\columnwidth]{./experiments/RedHVTPreferenceSPDeterministic/BlueMSNDeterministic/TreeNetwork40/results/report_plots/gido/hvt_CMs.pdf}
    }

    \subfloat[\treeFifty]{
    \label{fig:RedHVTPreferenceSPDeterministic:BlueMSNDeterministic:TreeNetwork50:hvt_CMs:gido}
    \includegraphics[width=0.8\columnwidth]{./experiments/RedHVTPreferenceSPDeterministic/BlueMSNDeterministic/TreeNetwork50/results/report_plots/gido/hvt_CMs.pdf}
    }

    \subfloat[\treeSeventy]{
    \label{fig:RedHVTPreferenceSPDeterministic:BlueMSNDeterministic:TreeNetwork70:hvt_CMs:gido}
    \includegraphics[width=0.8\columnwidth]{./experiments/RedHVTPreferenceSPDeterministic/BlueMSNDeterministic/TreeNetwork70/results/report_plots/gido/hvt_CMs.pdf}
    }

    \subfloat[\treeNinety]{
    \label{fig:RedHVTPreferenceSPDeterministic:BlueMSNDeterministic:TreeNetwork90:hvt_CMs:gido}
    \includegraphics[width=0.8\columnwidth]{./experiments/RedHVTPreferenceSPDeterministic/BlueMSNDeterministic/TreeNetwork90/results/report_plots/gido/hvt_CMs.pdf}
    }

    \subfloat[\treeMixed]{
    \label{fig:RedHVTPreferenceSPDeterministic:BlueMSNDeterministic:TreeNetworkMixed:hvt_CMs:gido}
    \includegraphics[width=0.8\columnwidth]{./experiments/RedHVTPreferenceSPDeterministic/BlueMSNDeterministic/TreeNetworkMixed/results/report_plots/gido/hvt_CMs.pdf}
    }

    \caption{Confusion matrices for for \hvt predictions (\gido).}
    \label{fig:treenets:cm_hvt:gido}
\end{figure}

\subsection*{High-Value User Confusion Matrices for \gido} \label{appendix:gido:results:hvu_cm}

\begin{figure}[H]
\centering

\subfloat[\treeThirty]{
\label{fig:RedHVTPreferenceSPDeterministic:BlueMSNDeterministic:TreeNetwork30:hvu_CMs:gido}
\includegraphics[width=0.8\columnwidth]{./experiments/RedHVTPreferenceSPDeterministic/BlueMSNDeterministic/TreeNetwork30/results/report_plots/gido/service_CMs.pdf}
}

\subfloat[\treeForty]{
\label{fig:RedHVTPreferenceSPDeterministic:BlueMSNDeterministic:TreeNetwork40:hvu_CMs:gido}
\includegraphics[width=0.8\columnwidth]{./experiments/RedHVTPreferenceSPDeterministic/BlueMSNDeterministic/TreeNetwork40/results/report_plots/gido/service_CMs.pdf}
}

\subfloat[\treeFifty]{
\label{fig:RedHVTPreferenceSPDeterministic:BlueMSNDeterministic:TreeNetwork50:hvu_CMs:gido}
\includegraphics[width=0.8\columnwidth]{./experiments/RedHVTPreferenceSPDeterministic/BlueMSNDeterministic/TreeNetwork50/results/report_plots/gido/service_CMs.pdf}
}

\subfloat[\treeSeventy]{
\label{fig:RedHVTPreferenceSPDeterministic:BlueMSNDeterministic:TreeNetwork70:hvu_CMs:gido}
\includegraphics[width=0.8\columnwidth]{./experiments/RedHVTPreferenceSPDeterministic/BlueMSNDeterministic/TreeNetwork70/results/report_plots/gido/service_CMs.pdf}
}

\subfloat[\treeNinety]{
\label{fig:RedHVTPreferenceSPDeterministic:BlueMSNDeterministic:TreeNetwork90:hvu_CMs:gido}
\includegraphics[width=0.8\columnwidth]{./experiments/RedHVTPreferenceSPDeterministic/BlueMSNDeterministic/TreeNetwork90/results/report_plots/gido/service_CMs.pdf}
}

\subfloat[\treeMixed]{
\label{fig:RedHVTPreferenceSPDeterministic:BlueMSNDeterministic:TreeNetworkMixed:hvu_CMs:gido}
\includegraphics[width=0.8\columnwidth]{./experiments/RedHVTPreferenceSPDeterministic/BlueMSNDeterministic/TreeNetworkMixed/results/report_plots/gido/service_CMs.pdf}
}

\caption{Confusion matrices for high-value user predictions (\gido).}
\label{fig:treenets:cm_hvu:gido}
\end{figure}

\subsection*{Character Network Embeddings Visualization for \gido} \label{appendix:gido:results:charnet_embeddings}

\begin{figure}[H]
\centering
\subfloat[\treeThirty]{
\label{fig:RedHVTPreferenceSPDeterministic:BlueMSNDeterministic:TreeNetwork30:correct_only_false:gido}
\includegraphics[width=\columnwidth]{./experiments/RedHVTPreferenceSPDeterministic/BlueMSNDeterministic/TreeNetwork30/results/report_plots/gido/charnet_embeddings_service_preference_correct_only_False.pdf}
}

\subfloat[\treeForty]{
\label{fig:RedHVTPreferenceSPDeterministic:BlueMSNDeterministic:TreeNetwork40:correct_only_false:gido}
\includegraphics[width=\columnwidth]{./experiments/RedHVTPreferenceSPDeterministic/BlueMSNDeterministic/TreeNetwork40/results/report_plots/gido/charnet_embeddings_service_preference_correct_only_False.pdf}
}

\subfloat[\treeFifty]{
\label{fig:RedHVTPreferenceSPDeterministic:BlueMSNDeterministic:TreeNetwork50:correct_only_false:gido}
\includegraphics[width=\columnwidth]{./experiments/RedHVTPreferenceSPDeterministic/BlueMSNDeterministic/TreeNetwork50/results/report_plots/gido/charnet_embeddings_service_preference_correct_only_False.pdf}
}

\subfloat[\treeSeventy]{
\label{fig:RedHVTPreferenceSPDeterministic:BlueMSNDeterministic:TreeNetwork70:correct_only_false:gido}
\includegraphics[width=\columnwidth]{./experiments/RedHVTPreferenceSPDeterministic/BlueMSNDeterministic/TreeNetwork70/results/report_plots/gido/charnet_embeddings_service_preference_correct_only_False.pdf}
}

\subfloat[\treeNinety]{
\label{fig:RedHVTPreferenceSPDeterministic:BlueMSNDeterministic:TreeNetwork90:correct_only_false:gido}
\includegraphics[width=\columnwidth]{./experiments/RedHVTPreferenceSPDeterministic/BlueMSNDeterministic/TreeNetwork90/results/report_plots/gido/charnet_embeddings_service_preference_correct_only_False.pdf}
}

\subfloat[\treeMixed]{
\label{fig:RedHVTPreferenceSPDeterministic:BlueMSNDeterministic:TreeNetworkMixed:correct_only_false:gido}
\includegraphics[width=\columnwidth]{./experiments/RedHVTPreferenceSPDeterministic/BlueMSNDeterministic/TreeNetworkMixed/results/report_plots/gido/charnet_embeddings_service_preference_correct_only_False.pdf}
}

\caption{Embedding plots from runs conducted across different \tree topologies.
For the last row, \treeMixed, data was gathered using all of the above
network topologies.}
\label{fig:results:treenet_embeddings:correct_only_false:gido}
\end{figure}

\begin{figure}[H]
\centering
\subfloat[\treeThirty]{
\label{fig:RedHVTPreferenceSPDeterministic:BlueMSNDeterministic:TreeNetwork30:correct_only_true:gido}
\includegraphics[width=\columnwidth]{./experiments/RedHVTPreferenceSPDeterministic/BlueMSNDeterministic/TreeNetwork30/results/report_plots/gido/charnet_embeddings_service_preference_correct_only_True.pdf}
}

\subfloat[\treeForty]{
\label{fig:RedHVTPreferenceSPDeterministic:BlueMSNDeterministic:TreeNetwork40:correct_only_true:gido}
\includegraphics[width=\columnwidth]{./experiments/RedHVTPreferenceSPDeterministic/BlueMSNDeterministic/TreeNetwork40/results/report_plots/gido/charnet_embeddings_service_preference_correct_only_True.pdf}
}

\subfloat[\treeFifty]{
\label{fig:RedHVTPreferenceSPDeterministic:BlueMSNDeterministic:TreeNetwork50:correct_only_true:gido}
\includegraphics[width=\columnwidth]{./experiments/RedHVTPreferenceSPDeterministic/BlueMSNDeterministic/TreeNetwork50/results/report_plots/gido/charnet_embeddings_service_preference_correct_only_True.pdf}
}

\subfloat[\treeSeventy]{
\label{fig:RedHVTPreferenceSPDeterministic:BlueMSNDeterministic:TreeNetwork70:correct_only_true:gido}
\includegraphics[width=\columnwidth]{./experiments/RedHVTPreferenceSPDeterministic/BlueMSNDeterministic/TreeNetwork70/results/report_plots/gido/charnet_embeddings_service_preference_correct_only_True.pdf}
}

\subfloat[\treeNinety]{
\label{fig:RedHVTPreferenceSPDeterministic:BlueMSNDeterministic:TreeNetwork90:correct_only_true:gido}
\includegraphics[width=\columnwidth]{./experiments/RedHVTPreferenceSPDeterministic/BlueMSNDeterministic/TreeNetwork90/results/report_plots/gido/charnet_embeddings_service_preference_correct_only_True.pdf}
}

\subfloat[\treeMixed]{
\label{fig:RedHVTPreferenceSPDeterministic:BlueMSNDeterministic:TreeNetworkMixed:correct_only_true:gido}
\includegraphics[width=\columnwidth]{./experiments/RedHVTPreferenceSPDeterministic/BlueMSNDeterministic/TreeNetworkMixed/results/report_plots/gido/charnet_embeddings_service_preference_correct_only_True.pdf}
}

\caption{Embedding plots from runs conducted across different tree network architectures,
but in contrast to \autoref{fig:results:treenet_embeddings:correct_only_false:gido} we exclude
the embeddings belonging to samples that were misclassified with respect to the user prediction.
The last row, \treeMixed, represents training runs where a \gido was trained on all of the above
network topologies (\treeThirty -- \treeNinety).}
\label{fig:results:treenet_embeddings:correct_only_true:gido}
\end{figure}
