# Supplementary material for: Machine Theory of Mind for Autonomous Cyber-Defence
Source: arXiv:2412.04367 source file (2024-12-05)
Supplement: Supplementary file 2 [file gigo.tex]

\section{\gigo results} \label{appendix:gigo:results}

\subsection*{Convergence Plots for \gigo} \label{appendix:gigo:results:convergence_plots}

\begin{figure}[H]
\centering
\includegraphics[width=0.9\columnwidth]{./experiments/RedHVTPreferenceSPDeterministic/BlueMSNDeterministic/TreeNetwork30/results/report_plots/gigo/convergence_plots_legend.pdf}

\subfloat[\treeThirty]{
\label{fig:RedHVTPreferenceSPDeterministic:BlueMSNDeterministic:TreeNetwork30:convergence_plots:gigo}
\includegraphics[width=0.9\columnwidth]{./experiments/RedHVTPreferenceSPDeterministic/BlueMSNDeterministic/TreeNetwork30/results/report_plots/gigo/convergence_plots.pdf}
}

\subfloat[\treeFifty]{
\label{fig:RedHVTPreferenceSPDeterministic:BlueMSNDeterministic:TreeNetwork50:convergence_plots:gigo}
\includegraphics[width=0.9\columnwidth]{./experiments/RedHVTPreferenceSPDeterministic/BlueMSNDeterministic/TreeNetwork50/results/report_plots/gigo/convergence_plots.pdf}
}

\subfloat[\treeNinety]{
\label{fig:RedHVTPreferenceSPDeterministic:BlueMSNDeterministic:TreeNetwork90:convergence_plots:gigo}
\includegraphics[width=0.9\columnwidth]{./experiments/RedHVTPreferenceSPDeterministic/BlueMSNDeterministic/TreeNetwork90/results/report_plots/gigo/convergence_plots.pdf}
}

\subfloat[\treeMixed]{
\label{fig:RedHVTPreferenceSPDeterministic:BlueMSNDeterministic:TreeNetworkMixed:convergence_plots:gigo}
\includegraphics[width=0.9\columnwidth]{./experiments/RedHVTPreferenceSPDeterministic/BlueMSNDeterministic/TreeNetworkMixed/results/report_plots/gigo/convergence_plots.pdf}
}

\caption{Convergence plots from our \tree runs. For each set of plots a \gido was trained data gathered on the respective \tree topology using \blueMSND and
\redHVTPreferenceSP agents.}
\label{fig:treenets:convergence:gigo}
\end{figure}

\subsection*{High-Value Target Confusion Matrices for \gigo} \label{appendix:gigo:results:hvt_cm}

\begin{figure}[H]
\centering
\subfloat[\treeThirty]{
\label{fig:RedHVTPreferenceSPDeterministic:BlueMSNDeterministic:TreeNetwork30:hvt_CMs:gigo}
\includegraphics[width=\columnwidth]{./experiments/RedHVTPreferenceSPDeterministic/BlueMSNDeterministic/TreeNetwork30/results/report_plots/gigo/hvt_CMs.pdf}
}

\subfloat[\treeFifty]{
\label{fig:RedHVTPreferenceSPDeterministic:BlueMSNDeterministic:TreeNetwork50:hvt_CMs:gigo}
\includegraphics[width=\columnwidth]{./experiments/RedHVTPreferenceSPDeterministic/BlueMSNDeterministic/TreeNetwork50/results/report_plots/gigo/hvt_CMs.pdf}
}

\subfloat[\treeNinety]{
\label{fig:RedHVTPreferenceSPDeterministic:BlueMSNDeterministic:TreeNetwork90:hvt_CMs:gigo}
\includegraphics[width=\columnwidth]{./experiments/RedHVTPreferenceSPDeterministic/BlueMSNDeterministic/TreeNetwork90/results/report_plots/gigo/hvt_CMs.pdf}
}

\subfloat[\treeMixed]{
\label{fig:RedHVTPreferenceSPDeterministic:BlueMSNDeterministic:TreeNetworkMixed:hvt_CMs:gigo}
\includegraphics[width=\columnwidth]{./experiments/RedHVTPreferenceSPDeterministic/BlueMSNDeterministic/TreeNetworkMixed/results/report_plots/gigo/hvt_CMs.pdf}
}
\caption{Confusion matrices for \hvt predictions (\gigo).}
\label{fig:treenets:cm_hvt:gigo}
\end{figure}

\newpage

\subsection*{Character Network Embeddings Visualization for \gigo} \label{appendix:gigo:results:charnet_embeddings}

\begin{figure}[H]
\centering
\subfloat[\treeThirty]{
\label{fig:RedHVTPreferenceSPDeterministic:BlueMSNDeterministic:TreeNetwork30:correct_only_false:gigo:pt1:appendix}
\includegraphics[width=0.24\columnwidth]{./experiments/RedHVTPreferenceSPDeterministic/BlueMSNDeterministic/TreeNetwork30/results/report_plots/gigo/charnet_embeddings_service_preference_Past_Trajectories__1_epoch150.pdf}
}
\subfloat[\treeThirty]{
\label{fig:RedHVTPreferenceSPDeterministic:BlueMSNDeterministic:TreeNetwork30:correct_only_false:gigo:pt2:appendix}
\includegraphics[width=0.24\columnwidth]{./experiments/RedHVTPreferenceSPDeterministic/BlueMSNDeterministic/TreeNetwork30/results/report_plots/gigo/charnet_embeddings_service_preference_Past_Trajectories__2_epoch150.pdf}
}
\subfloat[\treeThirty]{
\label{fig:RedHVTPreferenceSPDeterministic:BlueMSNDeterministic:TreeNetwork30:correct_only_false:gigo:pt3:appendix}
\includegraphics[width=0.24\columnwidth]{./experiments/RedHVTPreferenceSPDeterministic/BlueMSNDeterministic/TreeNetwork30/results/report_plots/gigo/charnet_embeddings_service_preference_Past_Trajectories__3_epoch150.pdf}
}
\subfloat[\treeThirty]{
\label{fig:RedHVTPreferenceSPDeterministic:BlueMSNDeterministic:TreeNetwork30:correct_only_false:gigo:pt4:appendix}
\includegraphics[width=0.24\columnwidth]{./experiments/RedHVTPreferenceSPDeterministic/BlueMSNDeterministic/TreeNetwork30/results/report_plots/gigo/charnet_embeddings_service_preference_Past_Trajectories__4_epoch150.pdf}
}

\subfloat[\treeFifty]{
\label{fig:RedHVTPreferenceSPDeterministic:BlueMSNDeterministic:TreeNetwork50:correct_only_false:gigo:pt1:appendix}
\includegraphics[width=0.24\columnwidth]{./experiments/RedHVTPreferenceSPDeterministic/BlueMSNDeterministic/TreeNetwork50/results/report_plots/gigo/charnet_embeddings_service_preference_Past_Trajectories__1_epoch150.pdf}
}
\subfloat[\treeFifty]{
\label{fig:RedHVTPreferenceSPDeterministic:BlueMSNDeterministic:TreeNetwork50:correct_only_false:gigo:pt2:appendix}
\includegraphics[width=0.24\columnwidth]{./experiments/RedHVTPreferenceSPDeterministic/BlueMSNDeterministic/TreeNetwork50/results/report_plots/gigo/charnet_embeddings_service_preference_Past_Trajectories__2_epoch150.pdf}
}
\subfloat[\treeFifty]{
\label{fig:RedHVTPreferenceSPDeterministic:BlueMSNDeterministic:TreeNetwork50:correct_only_false:gigo:pt3:appendix}
\includegraphics[width=0.24\columnwidth]{./experiments/RedHVTPreferenceSPDeterministic/BlueMSNDeterministic/TreeNetwork50/results/report_plots/gigo/charnet_embeddings_service_preference_Past_Trajectories__3_epoch150.pdf}
}
\subfloat[\treeFifty]{
\label{fig:RedHVTPreferenceSPDeterministic:BlueMSNDeterministic:TreeNetwork50:correct_only_false:gigo:pt4:appendix}
\includegraphics[width=0.24\columnwidth]{./experiments/RedHVTPreferenceSPDeterministic/BlueMSNDeterministic/TreeNetwork50/results/report_plots/gigo/charnet_embeddings_service_preference_Past_Trajectories__4_epoch150.pdf}
}

\subfloat[\treeNinety]{
\label{fig:RedHVTPreferenceSPDeterministic:BlueMSNDeterministic:TreeNetwork90:correct_only_false:gigo:pt1}
\includegraphics[width=0.24\columnwidth]{./experiments/RedHVTPreferenceSPDeterministic/BlueMSNDeterministic/TreeNetwork90/results/report_plots/gigo/charnet_embeddings_service_preference_Past_Trajectories__1_epoch150.pdf}
}
\subfloat[\treeNinety]{
\label{fig:RedHVTPreferenceSPDeterministic:BlueMSNDeterministic:TreeNetwork90:correct_only_false:gigo:pt2}
\includegraphics[width=0.24\columnwidth]{./experiments/RedHVTPreferenceSPDeterministic/BlueMSNDeterministic/TreeNetwork90/results/report_plots/gigo/charnet_embeddings_service_preference_Past_Trajectories__2_epoch150.pdf}
}
\subfloat[\treeNinety]{
\label{fig:RedHVTPreferenceSPDeterministic:BlueMSNDeterministic:TreeNetwork90:correct_only_false:gigo:pt3}
\includegraphics[width=0.24\columnwidth]{./experiments/RedHVTPreferenceSPDeterministic/BlueMSNDeterministic/TreeNetwork90/results/report_plots/gigo/charnet_embeddings_service_preference_Past_Trajectories__3_epoch150.pdf}
}
\subfloat[\treeNinety]{
\label{fig:RedHVTPreferenceSPDeterministic:BlueMSNDeterministic:TreeNetwork90:correct_only_false:gigo:pt4}
\includegraphics[width=0.24\columnwidth]{./experiments/RedHVTPreferenceSPDeterministic/BlueMSNDeterministic/TreeNetwork90/results/report_plots/gigo/charnet_embeddings_service_preference_Past_Trajectories__4_epoch150.pdf}
}

\subfloat[\treeMixed]{
\label{fig:RedHVTPreferenceSPDeterministic:BlueMSNDeterministic:TreeNetworkMixed:correct_only_false:gigo:pt1}
\includegraphics[width=0.24\columnwidth]{./experiments/RedHVTPreferenceSPDeterministic/BlueMSNDeterministic/TreeNetworkMixed/results/report_plots/gigo/charnet_embeddings_service_preference_Past_Trajectories__1_epoch150.pdf}
}
\subfloat[\treeMixed]{
\label{fig:RedHVTPreferenceSPDeterministic:BlueMSNDeterministic:TreeNetworkMixed:correct_only_false:gigo:pt2}
\includegraphics[width=0.24\columnwidth]{./experiments/RedHVTPreferenceSPDeterministic/BlueMSNDeterministic/TreeNetworkMixed/results/report_plots/gigo/charnet_embeddings_service_preference_Past_Trajectories__2_epoch150.pdf}
}
\subfloat[\treeMixed]{
\label{fig:RedHVTPreferenceSPDeterministic:BlueMSNDeterministic:TreeNetworkMixed:correct_only_false:gigo:pt3}
\includegraphics[width=0.24\columnwidth]{./experiments/RedHVTPreferenceSPDeterministic/BlueMSNDeterministic/TreeNetworkMixed/results/report_plots/gigo/charnet_embeddings_service_preference_Past_Trajectories__3_epoch150.pdf}
}
\subfloat[\treeMixed]{
\label{fig:RedHVTPreferenceSPDeterministic:BlueMSNDeterministic:TreeNetworkMixed:correct_only_false:gigo:pt4}
\includegraphics[width=0.24\columnwidth]{./experiments/RedHVTPreferenceSPDeterministic/BlueMSNDeterministic/TreeNetworkMixed/results/report_plots/gigo/charnet_embeddings_service_preference_Past_Trajectories__4_epoch150.pdf}
}

\caption{Embedding plots from runs conducted across different tree network architectures.
The last row, \treeMixed, represents training runs where a \gido was trained on all of the above
network topologies (\treeThirty -- \treeNinety).}
\label{fig:results:treenet_embeddings:correct_only_false:gigo}
\end{figure}
